# Supplementary material for: Transferable Adversarial Facial Images for Privacy Protection
Source: arXiv:2408.01428 source file (2024-07-18)
Supplement: Supplementary file 1 [file Supplementary.tex]

\documentclass[sigconf,review,anonymous]{acmart}
\usepackage{subfigure}
\usepackage{tabularray}
\usepackage{multirow}
\usepackage{booktabs}
\usepackage{colortbl}
\usepackage{algorithm}
\usepackage{algorithmic}

\settopmatter{printacmref=false} % Removes citation information below abstract
\renewcommand\footnotetextcopyrightpermission[1]{} % removes footnote with conference information in first column
\pagestyle{empty} % removes running headers
\acmSubmissionID{1922}

\setcopyright{acmcopyright}
\copyrightyear{2023}
\acmYear{2023}
\acmDOI{XXXXXXX.XXXXXXX}
%% These commands are for a PROCEEDINGS abstract or paper.
\acmConference[MM '24]{Proceedings of the 32nd ACM International Conference on Multimedia}{October 28 - November 1, 2024}{Melbourne, Australia}
\acmBooktitle{Proceedings of the 32nd ACM International Conference on Multimedia (MM '24), October 28 - November 1, 2024, Melbourne, Australia}
\acmPrice{15.00}
\acmISBN{978-1-4503-XXXX-X/18/06}

\begin{document}
\title{Transferable Adversarial Facial Images for Privacy Protection}

We sincerely thank the reviewers and would like to address the queries raised. 
\maketitle
\end{document}
